# Supplementary material for: Individual Control and Readout of Qubits in a Sub-Diffraction Volume
Source: arXiv:1805.06884 ancillary file (2018-08-20)
Supplement: Supplementary file 1 [file supplement-individual-control.pdf]

# Supplementary Information for "Individual Control and Readout of Qubits in a Sub-Diffraction Volume"

## S1. NITROGEN VACANCY STRAIN HAMILTONIAN

As derived by group theory [1, 2], the strain field contribution to the NV excited state Hamiltonian can be written in the basis of the NV excited states $\{E_1, E_2, E_x, E_y, A_1, A_2\}$:

$$H_{\text{str}} = \begin{pmatrix} \sigma_z & 0 & 0 & 0 & -\sigma_y & -\sigma_x \\ 0 & \sigma_z & 0 & 0 & \sigma_x & -\sigma_y \\ 0 & 0 & \sigma_z + \sigma_x & -\sigma_y & 0 & 0 \\ 0 & 0 & -\sigma_y & \sigma_z - \sigma_x & 0 & 0 \\ -\sigma_y & \sigma_x & 0 & 0 & \sigma_z & 0 \\ -\sigma_x & -\sigma_y & 0 & 0 & 0 & \sigma_z \end{pmatrix} \tag{S1}$$

The axial strain component $\sigma_z$ provides a simple uniform shift to all levels. While this does not affect the character of the levels, it can split nearby NVs experiencing differential axial strains. This is significant in our application, as an axial strain gradient would thus allow distinguishable NVs without the often associated spin mixing and coherence time degradation expected from higher strain samples.

The transverse component both splits (raising the levels $A_1, A_2, E_y$ and lowering the levels $E_1, E_2, E_x$) and mixes ($E_1$ with $\{A_1, A_2\}$, $E_2$ with $\{A_1, A_2\}$, and $E_x$ with $E_y$) the excited state manifold, resulting in two diverging spin triplet branches in the high strain limit.

## S2. SAMPLE PREPARATION

We use a PCD produced by CVD (Element Six) with a native nitrogen concentration of <50 ppb. To increase the prevalence of sub-diffraction clusters, the sample is implanted with nitrogen at 85 keV with a density of $10^{10}$ cm$^{-2}$, and subsequently annealed at 1200°C for 8 hours to heal the lattice and facilitate the formation of NV centers. To efficiently deliver microwaves to the sample, we fabricate gold striplines on the surface of the diamond using the following protocol:

1. Solvent clean, sonicating the sample in acetone, methanol, isopropyl alcohol (IPA), and water for 5 minutes each.
2. Oxygen plasma clean at 100 W for 5 minutes.
3. Spin-coat ZEP resist at 6 kRPM.
4. Write electron-beam patterns at 2 nA current, with a dose of 640 µC cm$^{-2}$.
5. Develop in ortho-xylene at room temperature for 10 seconds.
6. Deposit 5 nm of chrome for adhesion, followed by 100 nm of gold.
7. Sit overnight in N-Methyl-2-pyrrolidone (NMP) at room temperature.
8. Remove any remaining resist with sonication in NMP.
9. Clean with IPA.

The stripline is a simple loop with ends that taper out to large bonding pads. Figure S1a shows a camera image of two of these striplines post-fabrication. Figure S1b shows a confocal scan (532 nm) of the stripline used for these experiments, with a wire width of $w = 5$ µm and loop gap of $d = 30$ µm. Figure S1c is a close-up of the red boxed region of Figure S1b, showing a defect density that exhibits both clear single NVs and occasionally brighter clusters.

We perform wide-field spin echo measurements on a 25×25 µm$^2$ region of the PCD to characterize mean spin coherence time. Due to the randomized lattice orientation in each crystal grain, it is difficult to align a magnetic field to the NV axis, resulting in some off-axis field component that can degrade the coherence time [3]. Despite this, we measure a mean coherence time of $T_2 > 200$ µs (Fig. S2), indicating that NV centers in this sample maintain long coherence times despite the presence of high strain.

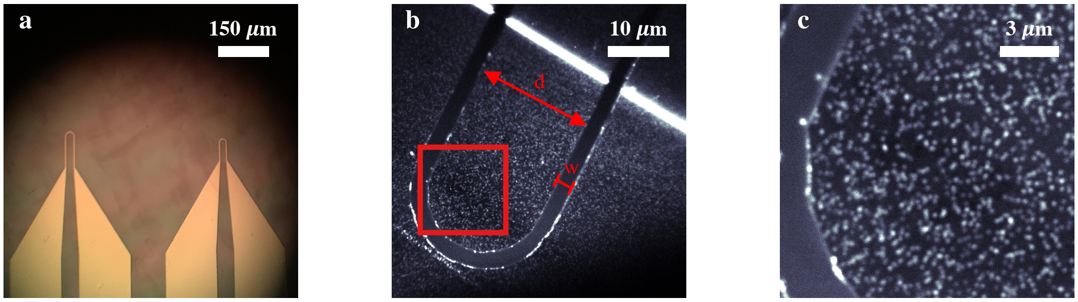


FIG. S1. **Striplines for microwave delivery.** **a**, Microscope camera image of striplines post-fabrication. **b**, Confocal image of a stripline on the PCD. The bright white line is a grain boundary in the diamond. The red box corresponds to the area scanned in **c**. For this stripline, $w = 5$ μm and $d = 30$ μm. **c**, A close-up of the red boxed area in **b**; this was the region used for the experiments described in the main texts.

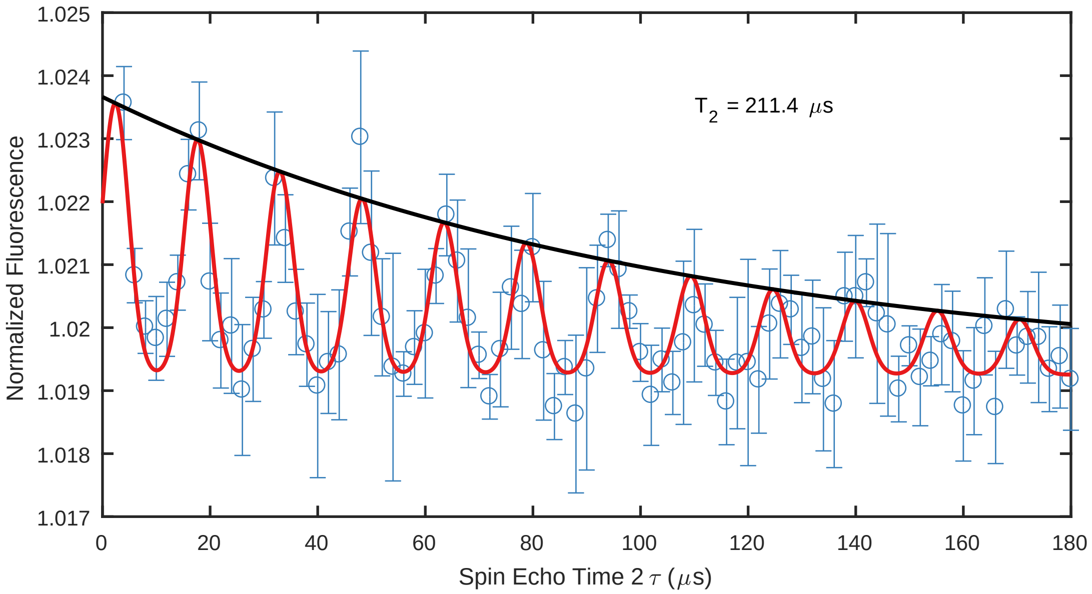


FIG. S2. **Coherence time characterization via spin echo measurements.** Averaged spin echo measurements taken on NV centers in a 25×25 μm$^2$ field of view on the PCD. Fitting the exponential decay of the revivals gives a mean coherence time of 211 μs

## S3. NV CLUSTER CHARACTERIZATION

As shown in Figure 1e of the main text, we measure seven prominent zero phonon line (ZPL) transitions in the PLE sweep. Our super resolution localization scans indicate that these correspond to three NVs; this is further corroborated by second-order autocorrelation measurements (Figure S3a), where the $g^{(2)}(0) = 0.728$ falls between 0.667 and 0.75, the $n = 3$ and $n = 4$ Fock state bounds respectively. In our PLE pulse sequence (see below), we start by initializing the NVs into their negatively charged, $m_s = 0$ spin state. Under perfect initialization and low spin-mixing, this state generally has two allowed transitions into $E_x$ and $E_y$ excited state manifolds. However, as discussed above in S1, highly strained systems can experience nontrivial mixing of the larger excited state manifold, yielding observation of more than the expected two transitions per NV center. We probe this using microwave application. Under an applied external magnetic field, we observe four optically detected magnetic resonance (ODMR) dips (Figure S3b), indicating that these three NVs have net two orientations (out of four possible). One resonance yields roughly twice as much contrast, indicating that two NVs fall along this orientation and one along the other. To determine which ODMR dips correspond to which NV centers, we apply microwaves at a single frequency corresponding to one of the spin

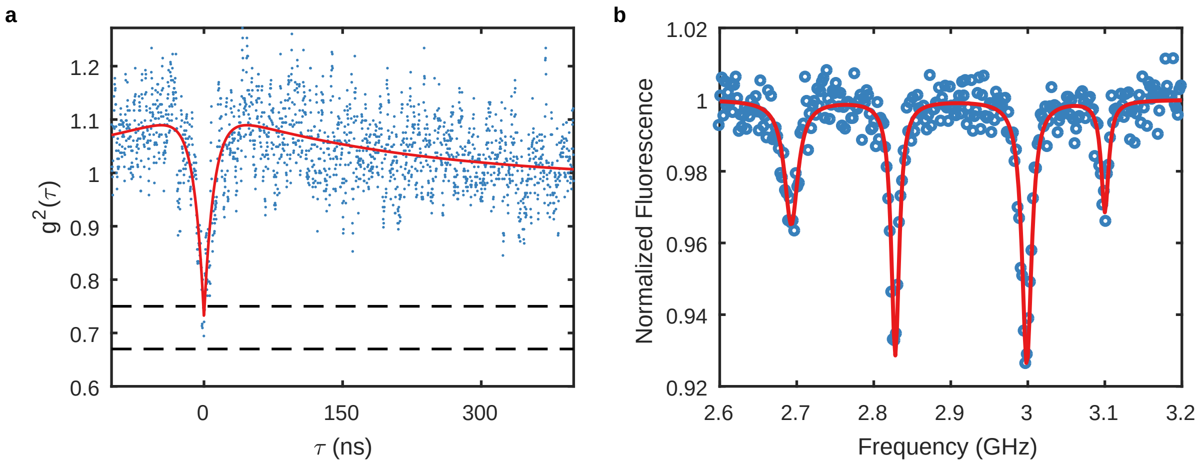


FIG. S3. **Characterization of NV cluster.** **a** Second-order autocorrelation measurement of the cluster system under 532 nm illumination. The red line is a fit to a model incorporating a bunching term, necessary due to the presence of shelving states of the NV. The dashed black lines mark the $n = 3$ (0.667) and $n = 4$ (0.75) photon bounds. **b**, ODMR of the cluster system under an applied external field. In the power-broadened regime, each NV orientation will exhibit at most two resonances, corresponding to the $m_s = 0 \Rightarrow m_s = \pm 1$ transitions. The observation of 4 thus indicates the presence of two orientations in the interrogated spot.

resonances, then selectively read out the system by collecting photon counts during application of a narrow laser locked to a single frequency corresponding to one of the ZPL resonances. If the microwave frequency and optical frequency are both resonant (with their respective transitions) for the same NV, then we expect to observe Rabi oscillations in fluorescence with varying microwave application times. If, however, the microwave frequency and optical frequency do not correspond to the same NV, then we expect to observe little to no modulation in fluorescence. Repeating this for each pairing of frequencies, we are able to map out which magnetic resonances come from which NVs, where we find indeed that two NVs correspond to the spin resonance with greater contrast. Furthermore, we are able to resolve the apparent extra ZPL transition; we find that while three of the ZPL peaks correspond to one spatial location (and thus one NV), one of these three (peak B in the main text) yields an increase in fluorescence under the microwave application described here, while all other transitions yield a decrease in fluorescence. This suggests that this extra peak is from a spin-mixed transition with both $m_s = 0$ and $m_s = 1$ character.

## S4. COUNT RATE AND CROSSTALK DERIVATION

As discussed in the main text, resonances of otherwise identical systems that are strain-split can experience preferential excitation (and thus fluorescence). In general, the steady-state excited level population of a two-level system with linewidth $\gamma$ under coherent excitation with Rabi frequency $\Omega$ at a detuning $\Delta$ is given by the optical Bloch equations to be:

$$\rho_{ee} = \frac{|\Omega|^2}{\left(\frac{\gamma}{2}\right)^2 + \Delta^2 + 2|\Omega|^2} \tag{S2}$$

For a pair of two-level systems with one on resonance, the ratio of their fluorescence rates is thus:

$$\frac{F_{resonant}}{F_{detuned}} = \frac{\left(\frac{\gamma}{2}\right)^2 + \Delta^2 + 2|\Omega|^2}{\left(\frac{\gamma}{2}\right)^2 + 2|\Omega|^2} \tag{S3}$$

$$\approx \frac{\Delta^2 + 2|\Omega|^2}{2|\Omega|^2} \tag{S4}$$

where the approximation in Eq. S4 is for the limiting case where $\Delta, |\Omega| \gg \gamma$. While this basic rate enhancement is sufficient for super-resolution localization and readout of an individual system, preservation of the off-resonant system's state requires more stringent conditions. We consider two types of crosstalk mechanisms; first, spin-projection errors that equate to a "measurement" of the off-resonant NV. For time scales shorter than the spin population decay

time $T_1$, we can treat the NV ground-excited states as a two-level system. During the resonant readout period, the off-resonant NV ($\Delta \gg \gamma$) undergoes Rabi oscillations:

$$\rho_{ee} = \frac{|\Omega|^2}{|\Omega|^2 + \Delta^2} \sin^2\left(t\sqrt{|\Omega|^2 + \Delta^2}\right) \tag{S5}$$

During this time, a decay from any small excited state population contribution constitutes a measurement of the system that degrades whatever initial spin superposition the NV originally had. In the limit for large detuning and short excitation times such that probability of spontaneous emission is $\ll 1$, this state has an expected number of decay events during a time $T$:

$$\lambda = \int_0^T \gamma\rho_{ee}dt \tag{S6}$$

$$= \frac{\gamma|\Omega|^2}{|\Omega|^2 + \Delta^2}\left[\frac{T}{2} - \frac{\sin\left(2T\sqrt{|\Omega|^2 + \Delta^2}\right)}{4\sqrt{|\Omega|^2 + \Delta^2}}\right] \tag{S7}$$

$$\approx \frac{\gamma|\Omega|^2 T}{2\left(|\Omega|^2 + \Delta^2\right)} \tag{S8}$$

where in the last line we take $T \gg \frac{1}{\sqrt{|\Omega|^2+\Delta^2}}$, which is appropriate for any non-pulsed measurement. Following Poissonian statistics, the probability $\Gamma$ of at least one decay event (crosstalk) occurring is then:

$$\Gamma = 1 - e^{-\gamma|\Omega|^2 T/2(|\Omega|^2+\Delta^2)} \tag{S9}$$

When considering the NV center's more complex level structure, we can generalize this result to a probability $\Gamma_{ijk}$ for a starting ground state $|i\rangle$, an excited level $|j\rangle$, and a final ground state $k$, yielding Equation 1 in the main text. Second, we consider phase errors resulting from differential AC Stark shift on the $|m_s = 0, 1\rangle$ spin ground states. The accumulated qubit phase error is given by the difference:

$$\phi = \frac{|E|^2}{\hbar}\left(\frac{\bar{\mu}_0^2}{\Delta_0} - \frac{\bar{\mu}_1^2}{\Delta_1}\right)t \tag{S10}$$

where each $\bar{\mu}_i$ is the projection on the field vector of the transition dipole for the spin $i$ ground-excited zero phonon line transition, and each $\Delta_i$ is the detuning of the near-resonant light from each respective transition. Typically, these transitions will be within ~10 GHz of one another, and the dipole moments roughly equal (though with different projections owing to the different polarizations of the transitions). To get a sense of the order of magnitude, we treat this in the case where $\Delta_1 \gg \Delta_0$, and note that this is a worse scenario than one would typically expect. We then see that the phase error goes simply with:

$$\phi \sim \frac{|\Omega|^2}{\Delta}t \tag{S11}$$

Taking typical experimental parameters of $|\Omega| \sim \gamma$, $\Delta \sim 10$ GHz, and $t \sim 100$ ns, this phase error is of order $10^{-2}$, and is thus not detectable in our experiment. We further note that under worse conditions, $|\Omega|$, $\Delta$, and $t$ can be well characterized and this phase error corrected.

## S5. PULSE SEQUENCES AND DATA ANALYSIS

### A. Localization Experiments

*Pulse sequences*

To measure PLE from individual NV centers, we use a pulse sequence consisting of a 5 µs 532 nm pulse to reionize and initialize the NVs into their $m_s = 0$ ground state, followed by a 10 µs pulse from our tunable red laser, during which time photon counts are collected on an avalanche photodiode. For the PLE measurement in Figure 1e, this is repeated $10^5$ times before retuning the frequency and repeating. For the super resolution localization experiments, the laser frequency is locked, and the sequence repeated $10^4$ times before moving to the next pixel in the scan.

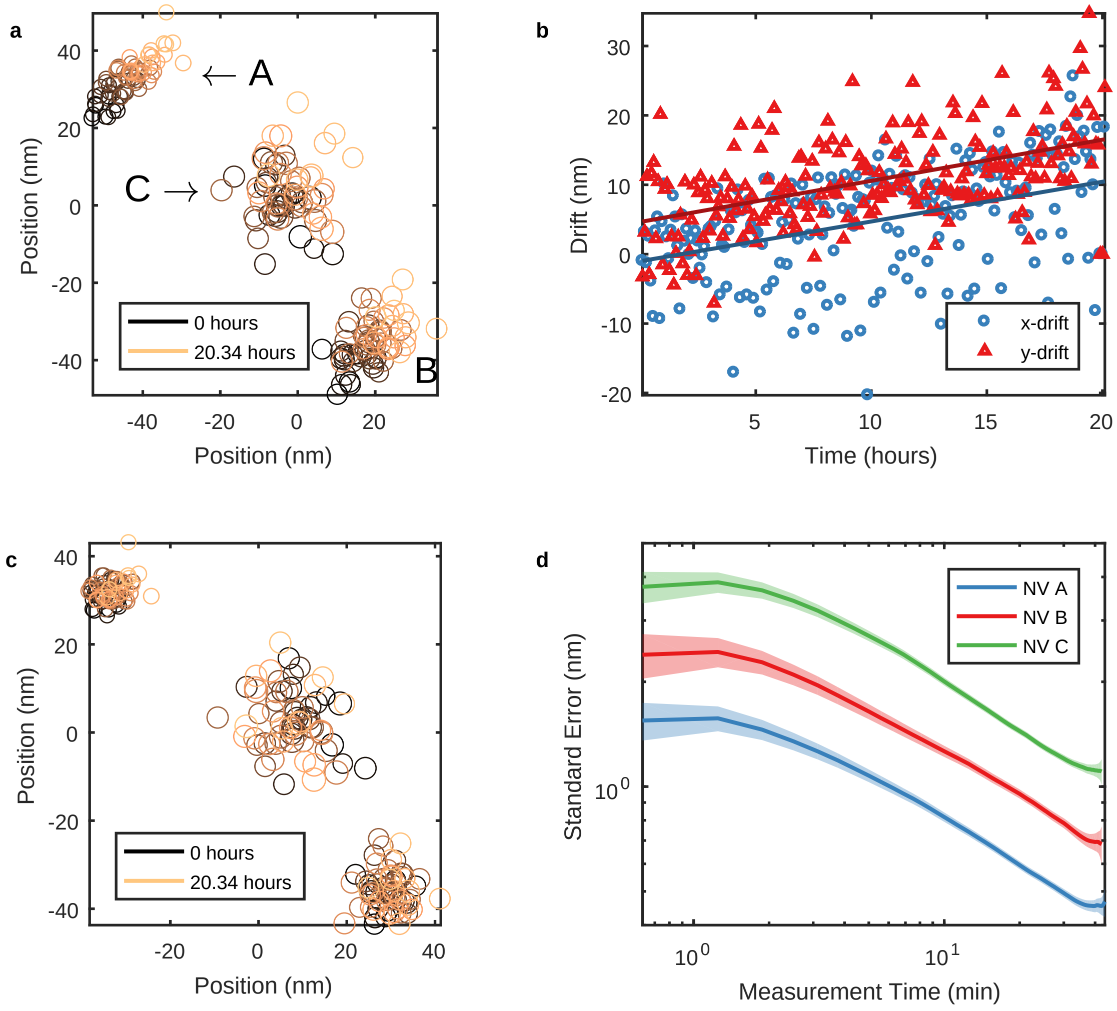


FIG. S4. **Super-resolution localization of individual NV centers.** **a**, Results of 69 super-resolution localization trials for each NV, with color representing the time at which the measurement was taking. Different NVs labeled by convention used above, and are given the same color scale, as the clusters are separated enough to distinguish by eye. Sizes of circles are in arbitrary units, but are scaled to indicate 95% confidence intervals on each measurement. **b**, Drift of all three NVs in $x$ (blue circles) and $y$ (red triangles) over the measurement period, overlaid with linear fits. **c**, Data from **a**, with drift compensated according to the fits in **b**. **d**, The standard error as per Equation S12 for each NV as a function of total measurement time.

### *Fitting and analysis*

For each NV, we repeat the resonant confocal scan 69 times over a period of around 20 hours, taking the spread on these Gaussian-fit centers from all experiments to be our true localization precision. The results of these individual trials are shown in Figures S4a, with the color gradient indicating relative time of each datapoint. As the data from each of the three NVs are well separated and clusters easily identifiable by eye, we plot each with the same color scheme.

Examining the temporal trend for each NV, it is readily apparent that there is some uniform drift on our stage over the course of the measurement period. In Figure S4b, for each NV, we plot the difference in $x$-coordinate and $y$-coordinate between the fit center at time $t$ and that at time $t = 0$. Both $x$ and $y$ follow clear trends, and linearly fitting these drifts allows us to compensate by shifting each datapoint's center according to the fitted drift for that time point. This adjustment results in the localization image shown in Figure S4c, clearly showing much tighter clustering than Figure S4a.

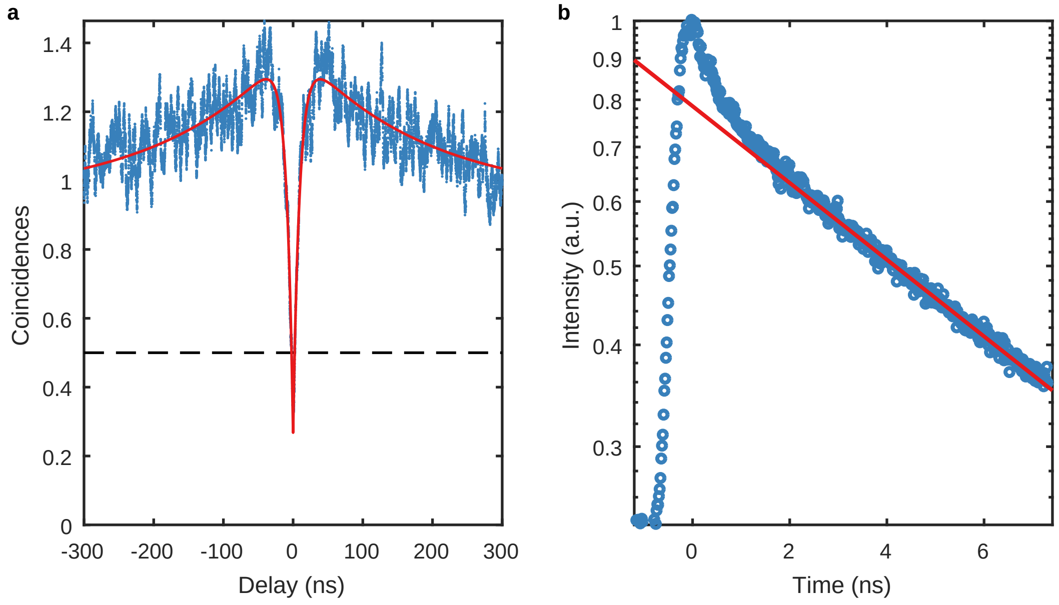


FIG. S5. **Characterization of single NV for detailed crosstalk measurements.** **a**, Second-order autocorrelation measurement taken with a Hanbury-Brown-Twiss interferometer. The coincidence dip below 0.5 at delay time $\tau = 0$ confirms that we are probing a single emitter. **b**, Lifetime measurements taken via pulsed excitation. The red line fitted to the decay after the initial instrument response yields an excited state lifetime of 9.2±0.1 ns.

From these data, we extract the standard distance, i.e. standard deviation in position, for each NV, dividing by $\sqrt{N}$ to convert to a standard error:

$$S(N) = \frac{1}{\sqrt{N}}\sqrt{\frac{\sum_{i=1}^{N}(x_i - \bar{x})^2 + (y_i - \bar{y})^2}{N}} \tag{S12}$$

where each $i$ is one of the 69 trials and $\bar{x}$ and $\bar{y}$ are mean positions of the total dataset (for a given NV). We calculate $S$ for every sequential binning of $N$ trials, with $N$ running from $N = 1$ to $N = N_{max} = 69$. Figure S4d plots the mean standard error as a function of total measurement time given by $T = Ndt$, where $dt = 37.5$ seconds is the total pulse sequence time to perform one scan experiment. Error bars indicate the standard error on the calculation of each $S(N)$. From these results, we demonstrate localization of single NV centers to a mean precision of 0.74 nm.

## B. Crosstalk Characterization Experiments

### *Single NV Characterization*

For verification of our crosstalk model, we perform Ramsey interferometry on a well-isolated single NV, verified by second-order autocorrelation measurements (Figure S5a), where a value $g^{(2)}(0) < 0.5$ indicates that a single photon emitter is being probed. An important parameter in the crosstalk model is the emitter lifetime. We characterize this on the single NV of interest by time-tagging photon counts after pulsed excitation, with results shown in Figure S5b. Fitting the decay after the initial instrument response yields a lifetime of 9.2±0.1 ns. We note that this is lower than the typical 12 ns lifetime commonly reported for NVs in a single-crystal bulk sample; this difference may stem from the presence of a particularly strained environment.

### *Fitting Ramsey Fringes*

As discussed in the main text, we experimentally probe off-resonant crosstalk by applying a near-resonant laser pulse of duration $T = 200$ ns during the precessionary period of a Ramsey interferometry sequence. In this case, crosstalk events manifest as decreased fringe contrast as the qubit is projected into an increasingly mixed state. To

fit these results, we first take a reference measurement of a Ramsey sequence with no crosstalk laser applied. The resultant fringes, shown in the last row of Figure 2b, are fit to a model with a decaying coherence envelope over three sinusoids corresponding to the three hyperfine transitions from coupling between the NV electronic spin and the nearby nitrogen-14 nuclear spin. Once this fit is retrieved, the data for varying crosstalk laser detunings (Figure 2b) are fit to this same equation, but with fixed decay envelope, sinusoid frequencies, phases, and relative amplitudes, leaving only one free parameter for the overall fringe amplitude, which gives the crosstalk probability.

That this crosstalk probability corresponds to the normalized Ramsey fringe amplitude is seen by considering the mixed state generated by the off-resonant pulse. In our Ramsey sequence, the spin is first optically polarized into the $m_s = 0$ spin state, then rotated by a $\pi/2$-pulse. In the $\{|m_s = 0\rangle, |m_s = 1\rangle, |m_s = -1\rangle\}$ basis, the density matrix for this process is:

$$\rho_{\text{initial}} = \begin{bmatrix} 1 & 0 & 0 \\ 0 & 0 & 0 \\ 0 & 0 & 0 \end{bmatrix} \xrightarrow{\pi/2} \frac{1}{2} \begin{bmatrix} 1 & 1 & 0 \\ 1 & 1 & 0 \\ 0 & 0 & 0 \end{bmatrix} \tag{S13}$$

The precession period then causes build-up of some phase $\theta(\tau)$. However, in the case of the off-resonant laser inducing a spontaneous emission event, the system's spin state is projected. The state at the end of this precession period can thus be written as a mixed state:

$$\rho_{\text{precession}} = \frac{(1-\Gamma)}{2} \begin{bmatrix} 1 & e^{-i\theta(\tau)} & 0 \\ e^{i\theta(\tau)} & 1 & 0 \\ 0 & 0 & 0 \end{bmatrix} + \Gamma_0 \begin{bmatrix} 1 & 0 & 0 \\ 0 & 0 & 0 \\ 0 & 0 & 0 \end{bmatrix} + \Gamma_1 \begin{bmatrix} 0 & 0 & 0 \\ 0 & 1 & 0 \\ 0 & 0 & 0 \end{bmatrix} + \Gamma_{-1} \begin{bmatrix} 0 & 0 & 0 \\ 0 & 0 & 0 \\ 0 & 0 & 1 \end{bmatrix}, \tag{S14}$$

where $\Gamma_k = \sum_{i,j} \Gamma_{ijk}$ is the probability of at least one spontaneous decay event into the $k$th ground state, and $\Gamma_0 + \Gamma_1 + \Gamma_{-1} = \Gamma$. The final $\pi/2$-pulse of the Ramsey sequence then produces the final state:

$$\rho_{\text{final}} = \frac{(1-\Gamma)}{2} \begin{bmatrix} 1-\cos(\theta(\tau)) & i\sin(\theta(\tau)) & 0 \\ -i\sin(\theta(\tau)) & 1+\cos(\theta(\tau)) & 0 \\ 0 & 0 & 0 \end{bmatrix} + \frac{\Gamma_0}{2} \begin{bmatrix} 1 & 1 & 0 \\ 1 & 1 & 0 \\ 0 & 0 & 0 \end{bmatrix} + \frac{\Gamma_1}{2} \begin{bmatrix} 1 & -1 & 0 \\ -1 & 1 & 0 \\ 0 & 0 & 0 \end{bmatrix} + \Gamma_{-1} \begin{bmatrix} 0 & 0 & 0 \\ 0 & 0 & 0 \\ 0 & 0 & 1 \end{bmatrix} \tag{S15}$$

At which point we measure the fluorescence under 532 nm illumination, which yields:

$$F_{\pi/2} = \left[\frac{(1-\Gamma)}{2}(1-\cos(\theta(\tau))) + \frac{\Gamma_0}{2} + \frac{\Gamma_1}{2}\right] F_0 + \left[\frac{(1+\Gamma)}{2}(1+\cos(\theta(\tau))) + \frac{\Gamma_0}{2} + \frac{\Gamma_1}{2}\right] F_1 + \Gamma_{-1} F_{-1}, \tag{S16}$$

where $F_i$ is the average fluorescence from the $|m_s = i\rangle$ state. For normalization over power fluctuations, we repeat this experiment, replacing the final $\pi/2$-pulse with a $3\pi/2$-pulse, which yields:

$$F_{3\pi/2} = \left[\frac{(1+\Gamma)}{2}(1+\cos(\theta(\tau))) + \frac{\Gamma_0}{2} + \frac{\Gamma_1}{2}\right] F_0 + \left[\frac{(1+\Gamma)}{2}(1-\cos(\theta(\tau))) + \frac{\Gamma_0}{2} + \frac{\Gamma_1}{2}\right] F_1 + \Gamma_{-1} F_{-1} \tag{S17}$$

Note that in both cases $F_1 = F_{-1}$. Using this, the contrast $C = \frac{(F_{3\pi/2} - F_{\pi/2})}{(F_{3\pi/2} + F_{\pi/2})}$ is then found to be:

$$C = \frac{(1-\Gamma)\cos(\theta(\tau))\,[F_1 - F_0]}{[F_1 + F_0] + \Gamma_{-1}\,[F_1 - F_0]} \tag{S18}$$

In our experiment, the $\Gamma_{-1}$ term is small ($\Gamma_{-1} \ll 1$), allowing us to simplify the above:

$$C = (1-\Gamma)\cos(\theta(\tau)) \frac{[F_1 - F_0]}{[F_1 + F_0]}, \tag{S19}$$

such that the time-varying fringe amplitude of the contrast in the main text is directly proportional to the crosstalk fidelity $(1-\Gamma)$. The correspondence between our model and the measured data in Figure 2c further supports that $\Gamma_{-1} \ll 1$.

### C. Simultaneous Control Experiments

*Logical green readout*

Due to experimental limitations in having only one red laser, we are forced to use non-selective 532 nm excitation to read the states of NVs A and B. In order to measure the states of NVs A and B in a way that is still independent of the state of NV C, we use a multi-pulse logical green readout. In this sequence, we first ionize NV C with a red pulse (2 µs) resonant with this NV's ZPL transition. To ensure ionization independent of the state of NV C, we further perform a $\pi$ MW pulse (32 ns) on this NV followed by another red pulse. The readout is then concluded by a 5 µs 532 nm pulse, where the first 500 ns are used for photon count collection and the remaining time is used to reset the charge state of the system.

*Pulse sequences*

The full pulse sequence used for the simultaneous control experiments described in the main text is shown Figure S6. As shown in Figure S6a, all spins are first initialized with a 5 µs 532 nm pulse. Next, a reference Ramsey measurement is taken on the two NVs of like orientation (NVs A and B) by applying a $\pi/2$ MW pulse (SMIQ06B, -9 dBm pre-amplifier, 42 ns), waiting for a free precession time $\tau$, then applying another $\pi/2$-pulse. Finally, we measure the state of these two NVs via a logical green readout, described in detail below.

After this reference Ramsey, the simultaneous control sequence in Figure S6b is performed. With all NVs initialized following the green readout, we first induce coherent Rabi oscillations in NV C by applying resonant MW (SMV03, 0 dBm pre-amplifier) for a time $\tau$. Next, we perform the same Ramsey pulse sequence as above; however, during the free precession period, we apply a red pulse resonant with the ZPL transition of NV C for a time $T = 300ns$ to read out its state, simultaneously collecting photon counts on an APD. After the second $\pi/2$-pulse concludes the Ramsey sequence, the system is read out with a logical green readout.

The next sets of pulses in Figure S6c are used for normalization. First, we perform our logical green readout to normalize the bright $m_s = 0$ state of all NVs. Next, we repeat the logical green readout, but with a $\pi$ pulse performed on NVs A and B in order to normalize the dark $m_s = 1$ states of these two NVs. Lastly, we repeat our red readout pulse to normalize to the bright state of NV C.

*Raw data analysis*

Figure S6d shows the raw counts divided by the appropriate normalization counts ($G$ for all Ramseys, $N$ for the Rabi), along with the fits described below.

We normalize the raw Rabi signal by dividing the counts retrieved during the $B$ bin by those retrieved during the red normalization bin $N$. This is fit with a model for Rabi oscillations with a sinusoidal envelope for the additional hyperfine interaction:

$$\text{Rabi} = [A_1 + A_2 \cos(\omega_1 \tau)] \cos(\omega_2 \tau - \phi) + C_B \tag{S20}$$

The fit minimum $A_1 + A_2$ is then used to normalize the counts to a population measurement as shown in the main text (Figure 3b).

The raw Ramsey counts (from both reference $R$ and simultaneous control $M$ signals) are normalized by the green $m_s = 0$ normalization bin $G$. These results are plotted in Figure S6d; for the main text, the reference (simultaneous control) signals are converted into a population measurement using the following normalization:

$$|c_0|^2 = \frac{R(M) - D}{G - D} \tag{S21}$$

This yields the results shown in Figure 3b. The reference Ramsey is fit to the following model, with three sinusoids for each of three hyperfine levels, as well as a decay term for the finite NV coherence time $T_2$:

$$\text{Ramsey} = e^{-\tau/T_2}\left[A_1 \cos(\omega_1 \tau - \phi_1) + A_2 \cos(\omega_2 \tau - \phi_2) + A_3 \cos(\omega_3 \tau - \phi_3)\right] + C_M \tag{S22}$$

For the simultaneous control Ramsey, due to infidelities in the $\pi$-pulse during the logical green readout, we see an additional signal from the Rabi on NV C corresponding to imperfect ionization of the $m_s = 1$ state. We thus fit this signal to the following model:

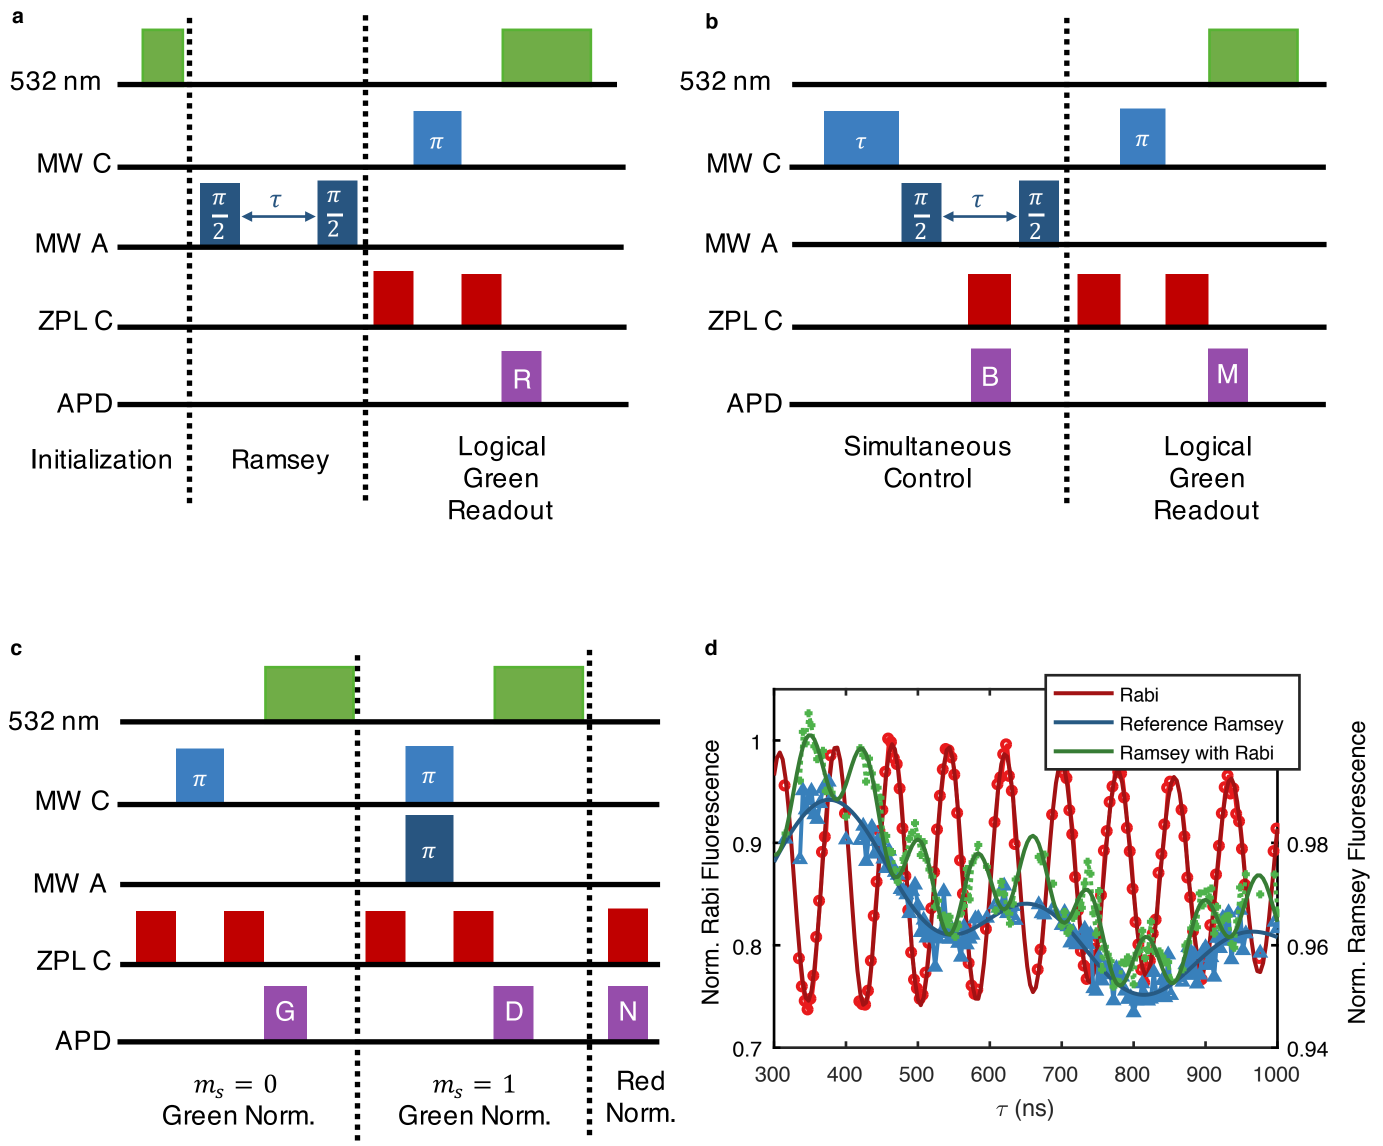


FIG. S6. **Full pulse sequence and results for simultaneous control experiments.** Sequences depicted in **a-c** were run end-to-end and repeated to yield the results shown in **d**. **a**, Sequence for reference Ramsey. **b**, Sequence for demonstrating simultaneous control by inducing Rabi oscillations on one spin population concurrent with a Ramsey sequence on another spin population. **c**, Sequences for normalizing the data collected in **a** and **b**. **d**, Fluorescence results normalized by the $m_s = 0$ green norm or red norm as appropriate, without any further modification.

$$S = A_1 \text{Ramsey} + C_M + A_2(1 - \text{Rabi}) \tag{S23}$$

Where the "Ramsey" and "Rabi" terms correspond to the fit results of the signal components of the above two models without offsets $C_B$ and $C_M$, and the $C_M$ term here is similarly not a fit parameter, but the same constant fit in the reference Ramsey. In this way, the only two fit parameters are the fidelity of the Ramsey signal $A_1$ and the relative contribution from the Rabi signal $A_2$, letting us determine the crosstalk. The crosstalk fidelity of our readout $(1 - \Gamma) = A_1$ is determined to be near unity at $A_1 = 1 \pm 0.04$, indicating that we have no detectable degradation of our signal as a result of the individual readout on NV C. This is consistent with our model; based on the known $\gamma = 13$ MHz, $\Omega = 1.7$ GHz, readout time $T = 300$ ns, and detuning $\Delta = 23$ GHz shown in Figure 1e, our model predicts a bit error probability of around 1%, below the 4% fit bounds. The residual difference between $S$ (data) and the reference Ramsey fit has a mean of 0.47%, further supporting our claim of crosstalk-free readout.

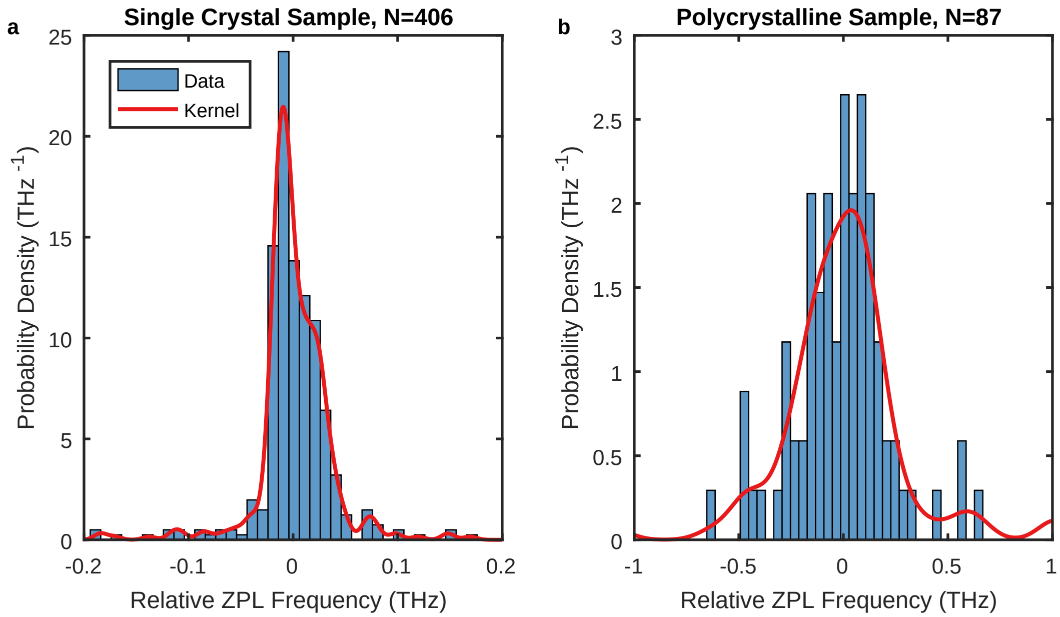


FIG. S7. **Comparison of datasets for empirically-determined inhomogeneous distributions of resonances.** **a**, Data and kernel estimate for the single-crystal sample. **b**, Data and kernel estimate for the polycrystalline sample. Note the difference in scaling of the horizontal axis.

### D. Empirical Zero-Phonon Line Distributions

The datasets for the empirical ZPL distributions are built by a multi-step sample characterization process, designed to minimize sampling bias by using low thresholding at each stage in order to ensure all potential candidates are fully investigated. First, a confocal fluorescence scan under 532 nm is taken, and bright peaks identified via coarse Gaussian image filtering and basic peak-finding. Second, the optical spectrum of each identified bright spot is taken, and analyzed for peaks in the range 636–638 nm. Finally, we perform high-resonant-power PLE measurements on all bright spots with identifiable spectral peaks. The use of high power here broadens the resonance lines, but does not change the central frequency, and ensures that even dimmer NVs will pass the threshold for peakfinding at this stage and be included in our final dataset. The empirical distributions for both the single-crystal and the polycrystalline samples are shown in Figure S7. As can be seen, the PCD exhibits a much broader distribution, which stems from the high-strain nature of the diverse grain structure. As the strain environment and corresponding ZPL distribution vary significantly between grains in the polycrystalline sample, we restrict our analysis to data from one representative grain, resulting in a lower number of datapoints compared to the single-crystal case.

[S1] M W Doherty, N B Manson, P Delaney, and L C L Hollenberg, "The negatively charged nitrogen-vacancy centre in diamond: the electronic solution," New Journal of Physics **13**, 025019 (2011).
[S2] J R Maze, A Gali, E Togan, Y Chu, A Trifonov, E Kaxiras, and M D Lukin, "Properties of nitrogen-vacancy centers in diamond: the group theoretic approach," New Journal of Physics **13**, 025025 (2011).
[S3] P. L. Stanwix, L. M. Pham, J. R. Maze, D. Le Sage, T. K. Yeung, P. Cappellaro, P. R. Hemmer, A. Yacoby, M. D. Lukin, and R. L. Walsworth, "Coherence of nitrogen-vacancy electronic spin ensembles in diamond," Phys. Rev. B **82**, 201201 (2010).
